# Supplementary material for: 103-Compound Band Structure Benchmark of Post-SCF Spin-Orbit Coupling Treatments in Density-Functional Theory
Source: arXiv:1705.01804 ancillary file (2017-07-10)
Supplement: Supplementary file 1 [file Huhn_2017_BandStructureBenchmark_SM.pdf]

# Supplemental Material for "103-Compound Band Structure Benchmark of Post-SCF Spin-Orbit Coupling Treatments in Density-Functional Theory"

William P. Huhn and Volker Blum

July 10, 2017

## 1 Introduction

In this document, we present the computational settings and materials used for the band structure benchmark including 103 materials incorporating 66 chemical species.

Two sets of calculated band structures are presented in this body of work, using two different sets of calculation parameters: "Benchmark Settings" and "Tight Production Settings". The main differences between these two settings are the density of the s.c.f. integration k-grid and the choice of basis sets. "Benchmark Settings" mimic the settings used in the Δ Project [11, 12] and are intended for comparison between FHI-aims [4] and Wien2k [3]. "Tight Production Settings" use sparser k-grids (though still reasonably well-sampled) and a smaller basis set (though still suitably large for accurate calculations of valence and low-lying conduction band) for comparison of band structures calculated using the semi-local PBE [15] and hybrid HSE06 [5, 6, 10] functionals by FHI-aims.

Input and output files (scalar-relativistic and spin-orbit-coupled) used in the band structure benchmark may be found on the NOMAD Repository [1]. Each set of band structure calculations has been assigned a Digital Object Identifier (DOI) suitable for citation. The band structure data set calculated by Wien2k using Benchmark Settings and the PBE functional is accessible at Ref. [7] The band structure data set calculated by FHI-aims using Benchmark Settings and the PBE functional is accessible at Ref. [8]

The band structure data set calculated by FHI-aims using Tight Production Settings and the HSE06 functional is accessible at Ref. [9] The related calculations performed using Tight Production Settings and the PBE functional are also included for comparison.

# 2 Computational Settings

## 2.1 FHI-aims Settings

A standard FHI-aims calculation requires two input files: a `geometry.in` file specifying the geometry of the material (lattice vectors + atomic coordinates) and a `control.in` file specifying the calculation parameters. In this section, we describe the contents of the `control.in` file. The contents of the `geometry.in` file may be found in Section 3.

We use "really_tight" integration settings for all FHI-aims benchmark calculations in this work. "Really_tight" integration settings are over-converged for practical calculations, and "tight" integration settings are recommended for production-quality calculations.

In this section, we describe the `control.in` file in detail.

### 2.1.1 FHI-aims, Benchmark Settings

Benchmark Settings have been constructed to guarantee well-converged calculations suitable for comparison between DFT codes on the semi-local level. All Benchmark Settings band structures presented have been calculated using the PBE functional. FHI-aims' "Tier 2" basis set is used for Benchmark Settings calculations performed with FHI-aims, consistent with the $\Delta$ Project. We generally calculate all eigenstates consistent with the chosen basis set and include them in second-variational spin-orbit coupling. The S.C.F. k-grid used by FHI-aims calculations using Benchmark Settings may be found in Section 2.3.

Calculations performed by FHI-aims using Benchmark Settings use the default convergence criterion for charge density; for all structures considered in this work, the default value will be 1.0d-6.

### 2.1.2 control.in Template, Benchmark Settings

A template for the `control.in` files used by FHI-aims for Benchmark Settings is provided here.

```
####################
# General Settings #
####################

# Run settings
restart wf
override_illconditioning .true.
basis_threshold 1E-7
calculate_all_eigenstates

# Periodic boundary conditions settings
k_grid  # [Material dependent; see text]
k_offset # [Material dependent;  see text]

# Physical model settings
xc pbe
charge 0.
```

```
spin none

# Relativistic settings
relativistic atomic_zora scalar
include_spin_orbit non_self_consistent

# SCF convergence settings
charge_mix_param 0.01
occupation_type gaussian 0.01
sc_iter_limit 300
sc_init_iter 301

# Relaxation settings

# Output options
output dos -20 30 1000 0.1

##################
# Band Structure #
##################
# K-paths taken from Setyawan and Curtarolo, 2010
# [See "Geometries and Band Structure K-Paths" for the k-paths used]

##############
# Basis Sets #
##############
# ["Tier 2" basis sets using "really tight" integration settings]
```

Ill-conditioning-related difficulties were encountered when using a Tier 2 basis set for the late transition metals Au, Ir, Pd, Pt, and Re. Accordingly, we made the follow modifications to `control.in` for these five elemental phases:

```
basis_threshold 1E-5
empty_states 100 # [Replaces "calculate_all_eigenstates"]
sc_iter_limit 1000
sc_init_iter 1001
```

We note that the resulting band structures show excellent agreement with Wien2k-calculated band structures on the scalar-relativistic level.

### 2.1.3 FHI-aims, Tight Production Settings

Tight Production Settings are constructed for comparison of band structures obtained from semi-local and hybrid calculations using computational settings that are production-quality. We continue using "really_tight" integration settings for Tight Production Settings, as real-space operations do not contribute significantly to the time and memory cost of a hybrid-functional calculation in FHI-aims.

Gamma-centered k-grids have been chosen for Tight Production Settings, that is, the `k_offset` keyword is omitted from the control.in file. Most calculations with Tight Production Settings were performed with an s.c.f. integration

k-grid of $16 \times 16 \times 16$. For 39 of the 103 materials, the k-grid density was modified. A list of the materials with different k-grids used is provided in Table S1. In most cases, the reduction in k-grid sampling is counterbalanced by a larger unit cell. Due to the expense of hybrid functional calculations, we manually specify the s.c.f. convergence criteria to values which are slightly looser than the default values set in FHI-aims but are known to be safe.

The default "tight" basis set in FHI-aims is used for all Tight Production Settings calculations. Default settings for the number of calculated eigenstates (commonly 35% to 75% of all possible eigenstates, see main text for more information) were used for materials with $Z \leq 79$ (Au). For materials with $Z \geq 80$ (Hg), the number of empty states (per atom) calculated and included in second-variational SOC was increased to 50.

HCP Co and BCC Fe have been omitted from the Tight Production data set, as we were unable to converge the electronic structure to the desired accuracy when using the HSE06 functional. We note in passing that convergence was quickly reached for the associated PBE calculations.

#### 2.1.4 control.in Template, Tight Production Settings

A template for the `control.in` files used by FHI-aims for Tight Production Settings is provided here.

```
####################
# General Settings #
####################

# Run settings
restart wf
override_illconditioning .true.
basis_threshold 1E-5

# Periodic boundary conditions settings
k_grid 16 16 16 # [See Table 1 for exceptions]

# Physical model settings
xc pbe # [See below for keywords used for HSE06 calculations]
charge 0.
spin none

# Relativistic settings
relativistic atomic_zora scalar
include_spin_orbit non_self_consistent

# Hybrid functionals settings
# [See below for keywords used for HSE06 calculations]

# SCF convergence settings
charge_mix_param 0.01
occupation_type gaussian 0.01
sc_accuracy_rho 1E-5
```

| Prototype | Chemical Formula | $N_1 N_2 N_3$ |
|---|---|---|
| GRA | C | 14 14 14 |
| WUR | AlN | 14 14 14 |
| HCP | Co | 14 14 10 |
| WUR | ZnS | 14 14 14 |
| HCP | Y | 14 14 14 |
| HCP | Zr | 14 14 14 |
| BCC | Nb | 14 14 14 |
| BCC | Mo | 14 14 14 |
| HCP | Tc | 14 14 14 |
| HCP | Ru | 14 14 14 |
| FCC | Rh | 14 14 14 |
| FCC | Pd | 14 14 14 |
| FCC | Ag | 14 14 14 |
| HCP | Cd | 14 14 14 |
| WUR | CdS | 14 14 10 |
| ZB | CdS | 14 14 14 |
| WUR | CdSe | 14 14 10 |
| ZB | CdSe | 14 14 14 |
| ZB | CdTe | 14 14 14 |
| WUR | InN | 14 14 14 |
| HCP | Lu | 14 14 10 |
| HCP | Hf | 14 14 10 |
| BCC | Ta | 12 12 12 |
| BCC | W | 12 12 12 |
| HCP | Re | 12 12 8 |
| HCP | Os | 12 12 8 |
| FCC | Ir | 12 12 12 |
| FCC | Pt | 12 12 12 |
| FCC | Au | 12 12 12 |
| ZB | HgS | 12 12 12 |
| ZB | HgSe | 12 12 12 |
| ZB | HgTe | 12 12 12 |
| HCP | Tl | 12 12 8 |
| FCC | Pb | 12 12 12 |
| RS | PbS | 12 12 12 |
| RS | PbSe | 12 12 12 |
| RS | PbTe | 12 12 12 |
| BCC | Bi | 12 12 12 |
| SCC | Po | 12 12 12 |

Table S1: Materials for which custom s.c.f. integration k-grids were used in Tight Production Settings for HSE06 calculations and their comparison to PBE. All materials not listed use a k-grid of $16 \times 16 \times 16$.

```
sc_accuracy_etot 1E-6
sc_accuracy_eev 1E-3
sc_iter_limit 300

# Relaxation settings

# Output options
output dos -20 30 1000 0.1

##################
# Band Structure #
##################
# K-paths taken from Setyawan and Curtarolo, 2010
# [See "Geometries and Band Structure K-Paths" for the k-paths used]

##############
# Basis Sets #
##############
# ["Tight" basis sets using "really tight" integration settings]
```

Based on the results of Appendix B, for materials with $Z \geq 80$ we increase the number of occupied states calculated and included in second-variational spin-orbit coupling via the additional keyword

```
empty_states 50
```

When performing a comparison of HSE06 and PBE calculations using Tight Production Settings, only the exchange-correlation functional used is varied; all other parameters (including the k-grid used) are left unchanged. For HSE06 calculations using FHI-aims, the keywords needed are:

```
xc hse06 0.2 # [Replaces "xc pbe" in the control.in stub]

# Hybrid functionals settings
hse_unit Angstrom-1
exx_band_structure_version 1
RI_method LVL_fast
```

## 2.2 Wien2k Settings

Computational settings for Wien2k calculations can be loosely grouped into two broad categories: species-specific settings (i.e. $R_{MT}$ and $RK_{max}$) and species-independent settings. All Wien2k calculations were performed with the PBE functional. Tight Production Settings are not presented for Wien2k, as we did not perform hybrid-functional calculations using Wien2k in this work. The version of Wien2k used was 14.2.

We note that here, as in the main text, we have abbreviated "(L)APW+lo self-consistent SOC" as "APW s.c. SOC", and similarly "(L)APW+lo self-consistent SOC including the $p^{1/2}$ orbital" as "APW+$p^{1/2}$ s.c. SOC"

### 2.2.1 Species-Specific Settings, Benchmark Settings

Table S2 lists $R_{MT}$ and $RK_{max}$ for the 66 chemical species contained in our data set (as well as He, Ar, and Kr which were omitted for the band structure benchmark, see Table S6). These settings generally correspond to the "WIEN2k/acc" settings from the $\Delta$ project [11, 12]. Notable exceptions include the Lu-Ir series, where ill-conditioning required that $RK_{max}$ be decreased. The $R_{MT}$'s of N, O, and F were increased, as these atoms occur exclusively in tetrahedrally-bonded semiconductors for this work. The resulting band structures show excellent quantitative agreement with FHI-aims for valence and low-lying conduction bands on the scalar-relativistic level (see Figure 5 of the main text and the discussion for more details.)

For materials containing two chemical species, a fixed value of $RK_{max}$=10 is used.

### 2.2.2 Species-Independent Settings, Benchmark Settings

In this section, we list Wien2k settings that were changed from their default values and do not (explicitly) depend on the chemical species used in the calculation.

The maximum l value for partial waves used inside atomic spheres (`lmax`) has been increased from 10 to 12. The maximum l value for partial waves used in the computation of non-muffin-tin matrix elements (`lnsmax`) has been increased from 4 to 6. An energy separation between core/valence states (`ecut`) of -9.0 Ry is used for all materials. An `EMAX` value of 10 Ry is used for SOC calculations.

The default Wien2k settings for charge and energy convergence (0.0001 e and 0.0001 Ry, respectively) were insufficient to guarantee electronic structure convergence for materials containing alkali and late transition metals. We use charge and energy convergence settings of 0.00001 e and 0.00001 Ry for all materials in this work.

The formulae for determination of s.c.f. k-grid used in Wien2k calculations are found in Section 2.3.

## 2.3 S.C.F. K-Grid for Benchmark Settings

The s.c.f. k-grid sampling (here denoted $N_1 \times N_2 \times N_3$) used by Wien2k and FHI-aims for Benchmark Settings calculations is given by the formulae:

$$N_1 = \texttt{ceiling}(\frac{\lambda\pi|k_B \times k_C|}{2V}) \tag{S1}$$

| Species | $R_{MT}$ | $RK_{max}$ | Species | $R_{MT}$ | $RK_{max}$ |
|---|---|---|---|---|---|
| He | 1.60 | 10.0 | Rb | 1.89 | 10.0 |
| Li | 1.60 | * (10.0) | Sr | 1.76 | 10.0 |
| Be | 1.80 | 10.0 | Y | 1.67 | 10.0 |
| B | 1.18 | * (7.5) | Zr | 1.60 | 10.0 |
| C | 1.10 | 7.5 | Nb | 1.60 | 10.0 |
| N | 1.49 (0.99) | * (7.5) | Mo | 1.60 | 10.0 |
| O | 1.20 (1.00) | * (7.5) | Tc | 1.60 | 10.0 |
| F | 1.50 (1.10) | * (8.0) | Ru | 1.60 | 10.0 |
| Ne | 1.60 | 10.0 | Rh | 1.60 | 10.0 |
| Na | 1.60 | * (10.0) | Pd | 1.60 | 10.0 |
| Mg | 1.60 | 10.0 | Ag | 1.60 | 10.0 |
| Al | 1.75 | 10.0 | Cd | 1.60 | 10.0 |
| Si | 1.57 | 10.0 | In | 1.98 | * (10.0) |
| P | 1.73 | * (10.0) | Sn | 1.88 | 10.0 |
| S | 1.60 | * (10.0) | Sb | 1.80 | * (10.0) |
| Cl | 1.60 | * (10.0) | Te | 2.17 | * (10.0) |
| Ar | 1.60 | 10.0 | I | 2.06 | * (10.0) |
| K | 1.60 | 10.0 | Xe | 2.00 | 10.0 |
| Ca | 1.60 | 10.0 | Cs | 1.70 (1.90) | 10.0 |
| Sc | 1.60 | 10.0 | Ba | 1.83 | 10.0 |
| Ti | 1.60 | 10.0 | Lu | 1.60 | 11.0 (12.0) |
| V | 1.60 | 10.0 | Hf | 1.60 | 11.0 (12.0) |
| Cr | 1.60 | 10.0 | Ta | 1.60 | 11.0 (12.0) |
| Mn | 1.60 | 10.0 | W | 1.60 | 11.0 (12.0) |
| Fe | 1.60 | 10.0 | Re | 1.60 | 11.0 (12.0) |
| Co | 1.93 | 11.0 (10.0) | Os | 1.60 | 11.0 (12.0) |
| Ni | 1.85 | 10.0 | Ir | 1.60 | 11.0 (12.0) |
| Cu | 1.78 | 10.0 | Pt | 1.77 (1.97) | 12.0 |
| Zn | 1.70 | 10.0 | Au | 1.87 | 12.0 |
| Ga | 2.04 | * (10.0) | Hg | 1.86 (2.06) | * (12.0) |
| Ge | 1.93 | 10.0 | Tl | 1.98 | 12.0 |
| As | 1.82 | * (10.0) | Pb | 1.91 | 12.0 |
| Se | 1.72 | * (10.0) | Bi | 1.85 | 12.0 |
| Br | 1.64 | * (10.0) | Po | 2.31 | 12.0 |
| Kr | 1.60 | 10.0 | | | |

Table S2: $R_{MT}$ and $RK_{max}$ used for Wien2k calculations. $RK_{max}$ for species appearing only in binaries have been marked with *, as all binaries use a fixed value of 10 for $RK_{max}$. In cases where settings have been changed from the "WIEN2k/acc" settings in the $\Delta$ project, the original value is specified in parentheses.

$$N_2 = \texttt{ceiling}(\frac{\lambda\pi|k_C \times k_A|}{2V}) \tag{S2}$$

$$N_3 = \texttt{ceiling}(\frac{\lambda\pi|k_A \times k_B|}{2V}) \tag{S3}$$

where $k_A$, $k_B$, and $k_C$ are the reciprocal lattice vectors of the unit cell, $V$ is the volume of the (direct) unit cell, and $\lambda$ is a free parameter for tuning the k-point density. We use $\lambda = 62$ in this work, as it gives k-grid densities comparable to the $\Delta$ project. We consistently use k-grids with even dimensions by incrementing all odd $N_i$.

A Monkhorst-Pack offset [13] is used for Benchmark Settings, which is automatically applied in Wien2k and may be applied in FHI-aims via the keyword `k_offset`.

# 3 Lattice Prototypes and Band Structure K-Paths

In this section, we present templates for the geometries used in the band structure benchmark, expressed in FHI-aims' `geometry.in` format. The geometries presented here may be converted into formats usable by other DFT codes via the OpenBabel tool. We also present the band structure k-paths for the corresponding Brillouin zone, expressed in an FHI-aims format but readily generalizable to other codes.

10 structural prototypes were used across the materials considered in this work: face-centered cubic, body-centered-cubic, simple cubic, (non-ideal) hexagonal close-packed, graphite, diamond, (cubic) zincblende, wurtzite, rocksalt, and CsCl. Within this class of 10 structural prototypes, there are a total of 5 possible material-dependent parameters: the standard crystallographic lattice parameters A and C, the species Element1 and Element2, and an additional internal degree of freedom Z for the wurtzite prototype.

We provide the k-paths used for band structure calculations in the form of FHI-aims keywords specified in `control.in`. We use the standardized k-paths proposed by Setyawan and Curarolo [17]. In an FHI-aims calculation, the k-path is specified by listing each individual branch of the k-path sequentially via the keyword

```
output band  k1_1 k1_2 k1_3  k2_1 k2_2 k2_3  NPOINTS k1 k2
```

where (k1_1, k1_2, k1_3) are the reciprocal coordinates of the initial k-point of the branch, (k2_1, k2_2, k2_3) are the reciprocal coordinates of the final k-point of the branch, NPOINTS is the number of k-points to be sampled along the branch (endpoints inclusive,) and k1 and k2 are strings used as labels for the initial and final k-points of the branch. All k-paths are given in the terms of the reciprocal lattice vectors of the associated direct unit cell. Identically sampled k-paths were used for Wien2k calculations.

We use 21 k-points per branch, as we find empirically that this resolution sufficiently samples fine features of the band structure.

## 3.1 Face-Centered Cubic (FCC)

### 3.1.1 geometry.in Template

```
lattice_vector     0  A/2  A/2
lattice_vector   A/2    0  A/2
lattice_vector   A/2  A/2    0
atom_frac          0    0    0  Element1
```

### 3.1.2 k-path Specified in control.in

```
output band  0.00000 0.00000 0.00000  0.50000 0.00000 0.50000   21 G X
output band  0.50000 0.00000 0.50000  0.50000 0.25000 0.75000   21 X W
output band  0.50000 0.25000 0.75000  0.37500 0.37500 0.75000   21 W K
output band  0.37500 0.37500 0.75000  0.00000 0.00000 0.00000   21 K G
output band  0.00000 0.00000 0.00000  0.50000 0.50000 0.50000   21 G L
output band  0.50000 0.50000 0.50000  0.62500 0.25000 0.62500   21 L U
output band  0.62500 0.25000 0.62500  0.50000 0.25000 0.75000   21 U W
```

```
output band  0.50000 0.25000 0.75000  0.50000 0.50000 0.50000   21 W L
output band  0.50000 0.50000 0.50000  0.37500 0.37500 0.75000   21 L K
output band  0.62500 0.25000 0.62500  0.50000 0.00000 0.50000   21 U X
```

## 3.2 Body-Centered Cubic (BCC)

### 3.2.1 geometry.in Template

```
lattice_vector   -A/2  A/2  A/2
lattice_vector    A/2 -A/2  A/2
lattice_vector    A/2  A/2 -A/2
atom_frac           0    0    0  Element1
```

### 3.2.2 k-path Specified in control.in

```
output band  0.00000  0.00000 0.00000  0.50000 -0.50000 0.50000   21 G H
output band  0.50000 -0.50000 0.50000  0.00000  0.00000 0.50000   21 H N
output band  0.00000  0.00000 0.50000  0.00000  0.00000 0.00000   21 N G
output band  0.00000  0.00000 0.00000  0.25000  0.25000 0.25000   21 G P
output band  0.25000  0.25000 0.25000  0.50000 -0.50000 0.50000   21 P H
output band  0.25000  0.25000 0.25000  0.00000  0.00000 0.50000   21 P N
```

## 3.3 Simple Cubic [Crystal] (SCC)

### 3.3.1 geometry.in Template

```
lattice_vector   A  0  0
lattice_vector   0  A  0
lattice_vector   0  0  A
atom_frac        0  0  0  Element1
```

### 3.3.2 k-path Specified in control.in

```
output band  0.00000 0.00000 0.00000  0.00000 0.50000 0.00000   21 G X
output band  0.00000 0.50000 0.00000  0.50000 0.50000 0.00000   21 X M
output band  0.50000 0.50000 0.00000  0.00000 0.00000 0.00000   21 M G
output band  0.00000 0.00000 0.00000  0.50000 0.50000 0.50000   21 G R
output band  0.50000 0.50000 0.50000  0.00000 0.50000 0.00000   21 R X
output band  0.50000 0.50000 0.00000  0.50000 0.50000 0.50000   21 M R
```

## 3.4 Hexagonal Close-Packed (HCP)

Note: We denote this prototype as HCP for simplicity, although we use non-ideal values for the crystallographic C parameter.

### 3.4.1 geometry.in Template

```
lattice_vector        A/2  -sqrt(3)*A/2         0
lattice_vector        A/2   sqrt(3)*A/2         0
lattice_vector          0             0         C
atom_frac               0             0         0  Element1
atom_frac        0.333333      0.666667  0.500000  Element1
```

### 3.4.2 k-path Specified in control.in

```
output band  0.00000 0.00000 0.00000  0.50000 0.00000 0.00000   21 G M
output band  0.50000 0.00000 0.00000  0.33333 0.33333 0.00000   21 M K
output band  0.33333 0.33333 0.00000  0.00000 0.00000 0.00000   21 K G
output band  0.00000 0.00000 0.00000  0.00000 0.00000 0.50000   21 G A
output band  0.00000 0.00000 0.50000  0.50000 0.00000 0.50000   21 A L
output band  0.50000 0.00000 0.50000  0.33333 0.33333 0.50000   21 L H
output band  0.33333 0.33333 0.50000  0.00000 0.00000 0.50000   21 H A
output band  0.50000 0.00000 0.50000  0.50000 0.00000 0.00000   21 L M
output band  0.33333 0.33333 0.00000  0.33333 0.33333 0.50000   21 K H
```

## 3.5 Graphite (GRA)

### 3.5.1 geometry.in Template

```
lattice_vector        A/2  -sqrt(3)*A/2         0
lattice_vector        A/2   sqrt(3)*A/2         0
lattice_vector          0             0         C
atom_frac        0.000000      0.000000   0.250000  Element1
atom_frac        0.000000      0.000000   0.750000  Element1
atom_frac       -0.333333      0.333333   0.250000  Element1
atom_frac        0.333333      0.666667   0.750000  Element1
```

### 3.5.2 k-path Specified in control.in

```
output band  0.00000 0.00000 0.00000  0.50000 0.00000 0.00000   21 G M
output band  0.50000 0.00000 0.00000  0.33333 0.33333 0.00000   21 M K
output band  0.33333 0.33333 0.00000  0.00000 0.00000 0.00000   21 K G
output band  0.00000 0.00000 0.00000  0.00000 0.00000 0.50000   21 G A
output band  0.00000 0.00000 0.50000  0.50000 0.00000 0.50000   21 A L
output band  0.50000 0.00000 0.50000  0.33333 0.33333 0.50000   21 L H
output band  0.33333 0.33333 0.50000  0.00000 0.00000 0.50000   21 H A
output band  0.50000 0.00000 0.50000  0.50000 0.00000 0.00000   21 L M
output band  0.33333 0.33333 0.00000  0.33333 0.33333 0.50000   21 K H
```

## 3.6 Diamond (DIA)

### 3.6.1 geometry.in Template

```
lattice_vector      0   A/2   A/2
lattice_vector    A/2     0   A/2
lattice_vector    A/2   A/2     0
atom_frac        0.00  0.00  0.00  Element1
atom_frac        0.25  0.25  0.25  Element1
```

### 3.6.2 k-path Specified in control.in

```
output band  0.00000 0.00000 0.00000  0.50000 0.00000 0.50000   21 G X
output band  0.50000 0.00000 0.50000  0.50000 0.25000 0.75000   21 X W
output band  0.50000 0.25000 0.75000  0.37500 0.37500 0.75000   21 W K
output band  0.37500 0.37500 0.75000  0.00000 0.00000 0.00000   21 K G
```

```
output band  0.00000 0.00000 0.00000  0.50000 0.50000 0.50000   21 G L
output band  0.50000 0.50000 0.50000  0.62500 0.25000 0.62500   21 L U
output band  0.62500 0.25000 0.62500  0.50000 0.25000 0.75000   21 U W
output band  0.50000 0.25000 0.75000  0.50000 0.50000 0.50000   21 W L
output band  0.50000 0.50000 0.50000  0.37500 0.37500 0.75000   21 L K
output band  0.62500 0.25000 0.62500  0.50000 0.00000 0.50000   21 U X
```

## 3.7 Cubic Zincblende (ZB)

### 3.7.1 geometry.in Template

```
lattice_vector      0   A/2   A/2
lattice_vector    A/2     0   A/2
lattice_vector    A/2   A/2     0
atom_frac        0.00  0.00  0.00  Element1
atom_frac        0.25  0.25  0.25  Element2
```

### 3.7.2 k-path Specified in control.in

```
output band  0.00000 0.00000 0.00000  0.50000 0.00000 0.50000   21 G X
output band  0.50000 0.00000 0.50000  0.50000 0.25000 0.75000   21 X W
output band  0.50000 0.25000 0.75000  0.37500 0.37500 0.75000   21 W K
output band  0.37500 0.37500 0.75000  0.00000 0.00000 0.00000   21 K G
output band  0.00000 0.00000 0.00000  0.50000 0.50000 0.50000   21 G L
output band  0.50000 0.50000 0.50000  0.62500 0.25000 0.62500   21 L U
output band  0.62500 0.25000 0.62500  0.50000 0.25000 0.75000   21 U W
output band  0.50000 0.25000 0.75000  0.50000 0.50000 0.50000   21 W L
output band  0.50000 0.50000 0.50000  0.37500 0.37500 0.75000   21 L K
output band  0.62500 0.25000 0.62500  0.50000 0.00000 0.50000   21 U X
```

## 3.8 Wurtzite (WUR)

### 3.8.1 geometry.in Template

```
lattice_vector        A/2  -sqrt(3)*A/2          0
lattice_vector        A/2   sqrt(3)*A/2          0
lattice_vector          0             0          C
atom_frac        0.666667      0.333333          0  Element1
atom_frac        0.333333      0.666667        0.5  Element1
atom_frac        0.666667      0.333333          Z  Element2
atom_frac        0.333333      0.666667      0.5+Z  Element2
```

### 3.8.2 k-path Specified in control.in

```
output band  0.00000 0.00000 0.00000  0.50000 0.00000 0.00000   21 G M
output band  0.50000 0.00000 0.00000  0.33333 0.33333 0.00000   21 M K
output band  0.33333 0.33333 0.00000  0.00000 0.00000 0.00000   21 K G
output band  0.00000 0.00000 0.00000  0.00000 0.00000 0.50000   21 G A
output band  0.00000 0.00000 0.50000  0.50000 0.00000 0.50000   21 A L
output band  0.50000 0.00000 0.50000  0.33333 0.33333 0.50000   21 L H
output band  0.33333 0.33333 0.50000  0.00000 0.00000 0.50000   21 H A
```

```
output band  0.50000 0.00000 0.50000  0.50000 0.00000 0.00000   21 L M
output band  0.33333 0.33333 0.00000  0.33333 0.33333 0.50000   21 K H
```

## 3.9 Rocksalt (RS)

### 3.9.1 geometry.in Template

```
lattice_vector     0  A/2  A/2
lattice_vector   A/2    0  A/2
lattice_vector   A/2  A/2    0
atom_frac          0    0    0  Element1
atom_frac        0.5  0.5  0.5  Element2
```

### 3.9.2 k-path Specified in control.in

```
output band  0.00000 0.00000 0.00000  0.50000 0.00000 0.50000   21 G X
output band  0.50000 0.00000 0.50000  0.50000 0.25000 0.75000   21 X W
output band  0.50000 0.25000 0.75000  0.37500 0.37500 0.75000   21 W K
output band  0.37500 0.37500 0.75000  0.00000 0.00000 0.00000   21 K G
output band  0.00000 0.00000 0.00000  0.50000 0.50000 0.50000   21 G L
output band  0.50000 0.50000 0.50000  0.62500 0.25000 0.62500   21 L U
output band  0.62500 0.25000 0.62500  0.50000 0.25000 0.75000   21 U W
output band  0.50000 0.25000 0.75000  0.50000 0.50000 0.50000   21 W L
output band  0.50000 0.50000 0.50000  0.37500 0.37500 0.75000   21 L K
output band  0.62500 0.25000 0.62500  0.50000 0.00000 0.50000   21 U X
```

## 3.10 Cesium Chloride (CSCL)

### 3.10.1 geometry.in Template

```
lattice_vector   A    0    0
lattice_vector   0    A    0
lattice_vector   0    0    A
atom_frac        0    0    0  Element1
atom_frac      0.5  0.5  0.5  Element2
```

### 3.10.2 k-path Specified in control.in

```
output band  0.00000 0.00000 0.00000  0.00000 0.50000 0.00000   21 G X
output band  0.00000 0.50000 0.00000  0.50000 0.50000 0.00000   21 X M
output band  0.50000 0.50000 0.00000  0.00000 0.00000 0.00000   21 M G
output band  0.00000 0.00000 0.00000  0.50000 0.50000 0.50000   21 G R
output band  0.50000 0.50000 0.50000  0.00000 0.50000 0.00000   21 R X
output band  0.50000 0.50000 0.00000  0.50000 0.50000 0.50000   21 M R
```

# 4 Materials Used and Structural Parameters

In this section, the 103 materials included in the band structure benchmark are listed. This set of materials is divided into three subsets: compound semiconductors (37 materials), elemental materials (45 materials), and alkali halides (21 materials.) Each material is specified by its structural prototype and the parameters needed for the given structural prototype (see Section 3). Units of Angstroms are used for lattice parameters.

In Table S6 we provide 8 materials that were considered for inclusion in the band structure benchmark but omitted. The materials excluded from the band structure benchmark due to overly large $\Delta_{band}$ values were alkali metals and (hypothetical) solid noble gas phases, but it is unclear to the authors at this time which code is primarily responsible for the disagreement.

## 4.1 Compound Semiconductors

Table S3 lists the materials included in the compound semiconductor subset. Most structures in this list are taken from Pearson's Handbook [19], but some were taken from Adachi [2] and other sources (where indicated).

## 4.2 Elemental Materials

Table S4 lists the materials included in the elemental materials subset. Elemental materials from the $\Delta$ Project with simple prototypes (FCC, BCC, HCP, graphite (GRA), diamond (DIA), or simple cubic [crystal] (SCC)) were chosen. Structural prototypes were chosen to match the T=0 phases used in the $\Delta$ Project (c.f. supplementary information of [12].) Experimentally reported lattice parameters were obtained from Pearson's Handbook [19], with the exception of hypothetical noble gas solids, where lattice parameters were obtained from Villars and Daam [20]. Pearson does not include structural parameters for the low-temperature hR6 structure used for Bi in the $\Delta$ Project, so a reported BCC phase for Bi is used instead.

## 4.3 Alkali Halides

Tables S5 lists the materials included in the alkali halides subset. All lattice parameters were taken from Wyckoff [21].

| Prototype | Element1 | Element2 | Source | A [Å] | C [Å] | Z |
|---|---|---|---|---|---|---|
| DIA | C | | Pearson | 3.5669 | | |
| RS | Mg | O | Pearson | 4.2147 | | |
| WUR | Al | N | Pearson | 3.110 | 4.980 | 0.382 |
| ZB | Al | N | Adachi | 4.38 | | |
| ZB | Si | C | Pearson | 4.358 | | |
| ZB | B | P | Adachi | 4.5383 | | |
| ZB | Al | P | Pearson | 5.4625 | | |
| RS | Mg | S | Pearson | 5.1913 | | |
| WUR | Zn | O | Pearson | 3.2499 | 5.2066 | 0.3825 |
| WUR | Zn | S | Pearson | 3.8225 | 6.261 | 0.371 |
| ZB | Zn | S | Pearson | 5.4109 | | |
| WUR | Ga | N | Pearson | 3.190 | 5.189 | 0.377 |
| ZB | Ga | N | Adachi | 4.52 | | |
| ZB | Ga | P | Pearson | 5.4504 | | |
| ZB | B | As | Pearson | 4.7667 | | |
| ZB | Al | As | Pearson | 5.660 | | |
| ZB | Ga | As | Pearson | 5.6532 | | |
| RS | Mg | Se | Pearson | 5.463 | | |
| ZB | Zn | Se | Pearson | 5.6670 | | |
| WUR | Cd | S | Pearson | 4.160 | 6.756 | 0.375 |
| ZB | Cd | S | Pearson | 5.832 | | |
| WUR | Cd | Se | Ref [18] | 4.2982 | 7.0084 | 0.3759 |
| ZB | Cd | Se | Pearson | 6.04 | | |
| WUR | In | N | Pearson | 3.540 | 5.704 | 0.375 |
| ZB | In | P | Pearson | 5.8687 | | |
| ZB | In | As | Pearson | 6.0584 | | |
| ZB | Al | Sb | Pearson | 6.1355 | | |
| ZB | Ga | Sb | Pearson | 6.0959 | | |
| ZB | In | Sb | Pearson | 6.4791 | | |
| ZB | Zn | Te | Ref. [14] | 6.1037 | | |
| ZB | Cd | Te | Pearson | 6.474 | | |
| ZB | Hg | S | Pearson | 5.874 | | |
| ZB | Hg | Se | Pearson | 6.0854 | | |
| ZB | Hg | Te | Pearson | 6.4588 | | |
| RS | Pb | S | Pearson | 5.9362 | | |
| RS | Pb | Se | Pearson | 6.1265 | | |
| RS | Pb | Te | Pearson | 6.4603 | | |

Table S3: Materials contained in the compound semiconductor subset of the band structure benchmark.

| Prototype | Element1 | Source | A [Å] | C [Å] |
|---|---|---|---|---|
| HCP | Be | Pearson | 2.2858 | 3.5843 |
| GRA | C | Pearson | 2.464 | 6.711 |
| FCC | Ne | Villars | 4.462 | |
| HCP | Mg | Pearson | 3.2089 | 5.2101 |
| FCC | Al | Pearson | 4.0488 | |
| DIA | Si | Pearson | 5.4286 | |
| FCC | Ca | Pearson | 5.5884 | |
| HCP | Sc | Pearson | 3.308 | 5.267 |
| HCP | Ti | Pearson | 2.9508 | 4.6855 |
| BCC | V | Pearson | 3.0271 | |
| BCC | Cr | Pearson | 2.884 | |
| FCC | Mn | Pearson | 3.862 | |
| BCC | Fe | Pearson | 2.8665 | |
| HCP | Co | Pearson | 2.5071 | 4.0695 |
| FCC | Ni | Pearson | 3.5232 | |
| FCC | Cu | Pearson | 3.6148 | |
| HCP | Zn | Pearson | 2.6646 | 4.9461 |
| DIA | Ge | Pearson | 5.6580 | |
| FCC | Sr | Pearson | 6.084 | |
| HCP | Y | Pearson | 3.6509 | 5.7388 |
| HCP | Zr | Pearson | 3.232 | 5.147 |
| BCC | Nb | Pearson | 3.3002 | |
| BCC | Mo | Pearson | 3.1470 | |
| HCP | Tc | Pearson | 2.7407 | 4.3980 |
| HCP | Ru | Pearson | 2.700 | 4.275 |
| FCC | Rh | Pearson | 3.8034 | |
| FCC | Pd | Pearson | 3.8874 | |
| FCC | Ag | Pearson | 4.0853 | |
| HCP | Cd | Pearson | 2.9787 | 5.6166 |
| DIA | Sn | Pearson | 6.4892 | |
| FCC | Xe | Villars | 6.350 | |
| BCC | Ba | Pearson | 5.013 | |
| HCP | Lu | Pearson | 3.5098 | 5.5666 |
| HCP | Hf | Pearson | 3.198 | 5.061 |
| BCC | Ta | Pearson | 3.3025 | |
| BCC | W | Pearson | 3.1652 | |
| HCP | Re | Pearson | 2.7609 | 4.4576 |
| HCP | Os | Pearson | 2.7353 | 4.3191 |
| FCC | Ir | Pearson | 3.8390 | |
| FCC | Pt | Pearson | 3.9242 | |
| FCC | Au | Pearson | 4.0789 | |
| HCP | Tl | Pearson | 3.4566 | 5.5248 |
| FCC | Pb | Pearson | 4.9507 | |
| BCC | Bi | Pearson | 3.800 | |
| SCC | Po | Pearson | 3.345 | |

Table S4: Materials contained in the elemental materials subset of the band structure benchmark.

| Prototype | Element1 | Element2 | Source | A [Å] |
|---|---|---|---|---|
| RS | Li | F | Wyckoff | 4.0173 |
| RS | Na | F | Wyckoff | 4.620 |
| RS | Li | Cl | Wyckoff | 5.12954 |
| RS | Na | Cl | Wyckoff | 5.64056 |
| RS | K | F | Wyckoff | 5.347 |
| RS | K | Cl | Wyckoff | 6.29294 |
| RS | Li | Br | Wyckoff | 5.5013 |
| RS | Na | Br | Wyckoff | 5.97324 |
| RS | K | Br | Wyckoff | 6.6000 |
| RS | Rb | F | Wyckoff | 5.64 |
| RS | Rb | Cl | Wyckoff | 6.5810 |
| RS | Rb | Br | Wyckoff | 6.854 |
| RS | Li | I | Wyckoff | 6.000 |
| RS | Na | I | Wyckoff | 6.4728 |
| RS | K | I | Wyckoff | 7.06555 |
| RS | Rb | I | Wyckoff | 7.342 |
| RS | Cs | F | Wyckoff | 6.008 |
| CSCL | Cs | Cl | Wyckoff | 4.123 |
| RS | Cs | Cl | Wyckoff | 7.02 |
| CSCL | Cs | Br | Wyckoff | 4.286 |
| CSCL | Cs | I | Wyckoff | 4.5667 |

Table S5: Materials contained in the alkali halides subset of the band structure benchmark.

| Prototype | Element1 | Element2 | Source | A [Å] | C [Å] | Rationale for Omission |
|---|---|---|---|---|---|---|
| HCP | He | | Villars | 3.555 | 5.798 | $\Delta_{band}$ of 2032 meV for low-lying conduction bands |
| ZB | B | N | Pearson | 3.6155 | | Failure to converge in Wien2k using Benchmark Settings |
| FCC | Ar | | Villars | 5.316 | | $\Delta_{band}$ of 238 meV for low-lying conduction bands |
| BCC | K | | Pearson | 5.3298 | | $\Delta_{band}$ of 57 meV for low-lying conduction bands |
| FCC | Kr | | Villars | 5.810 | | $\Delta_{band}$ of 103 meV for low-lying conduction bands |
| BCC | Rb | | Pearson | 5.699 | | $\Delta_{band}$ of 96 meV for low-lying conduction bands |
| RS | Mg | Te | Pearson | 6.026 | | Failure to converge in Wien2k using Benchmark Settings |
| BCC | Cs | | Pearson | 6.465 | | $\Delta_{band}$ of 110 meV for low-lying conduction bands |

Table S6: Materials which were considered for inclusion in the band structure benchmark but omitted. The rationale is provided in the final column. The definition of $\Delta_{band}$ may be found in the main text. We define low-lying conduction bands to be the set of states with energy eigenvalues lying in the energy window [CBM, CBM + 5 eV].

# 5 Results, Benchmark Settings

Tables S7, S8, and S9 list the spin-orbit splittings for select k-points obtained from FHI-aims and Wien2k band structures calculations using Benchmark Settings. To specify which spin-orbit splitting is being considered, we indicate the k-point where the spin-orbit splitting occurs alongside the energy eigenvalue of the associated scalar-relativistic eigenstates (i.e. the non-SOC-perturbed eigenvalue) for both FHI-aims and Wien2k.

"N/A" denotes either the spin-orbit splittings in the material were too weak to be visually distinguished in the energy range [VBM - 10 eV, VBM + 10 eV] or no unambiguous spin-orbit splitting (i.e. no single scalar-relativistic energy level clearly splitting into two spin-orbit-coupled energy levels) could be visually identified in the energy range. The exceptions are Ge, GaSb, and InS, where the overall spin-orbit splitting of the highest occupied band at $\Gamma$ is included in this set despite ambiguity for PBE calculations. For materials whose spin-orbit splittings show subband splitting (see Appendix B), the overall splitting of the band is used.

The zero of energy is set to the valence band maximum for insulators and the Fermi energy for metals. Units of eV are used for energies, and a conversion factor of 1 Ry = 13.60569225 eV has been used when converting energy eigenvalues calculated with Wien2k.

| Prototype | Material | K-Point | SR Energy Wien2k | SR Energy FHI-aims | SO Split APW | SO Splitting APW+p1/2 | SO Splitting NAO |
|---|---|---|---|---|---|---|---|
| DIA | C | N/A | | | | | |
| RS | MgO | N/A | | | | | |
| WUR | AlN | N/A | | | | | |
| ZB | AlN | N/A | | | | | |
| ZB | SiC | N/A | | | | | |
| ZB | BP | N/A | | | | | |
| ZB | AlP | Γ | 0 | 0 | 0.05987 | 0.05988 | 0.06008 |
| RS | MgS | Γ | 0 | 0 | 0.09349 | 0.09354 | 0.09255 |
| WUR | ZnO | H | -4.54699 | -4.54351 | 0.27668 | 0.27670 | 0.26921 |
| WUR | ZnS | Γ | 0 | 0 | 0.03172 | 0.03173 | 0.03124 |
| ZB | ZnS | Γ | 0 | 0 | 0.05911 | 0.05916 | 0.05906 |
| WUR | GaN | Γ | 9.88542 | 9.89604 | 0.20868 | 0.21183 | 0.22002 |
| ZB | GaN | N/A | | | | | |
| ZB | GaP | Γ | 3.89259 | 3.89120 | 0.16304 | 0.16521 | 0.16723 |
| ZB | BAs | Γ | 0 | 0 | 0.20445 | 0.20599 | 0.21041 |
| ZB | AlAs | Γ | 0 | 0 | 0.29513 | 0.29684 | 0.30203 |
| ZB | GaAs | Γ | 0 | 0 | 0.32954 | 0.33224 | 0.33963 |
| RS | MgSe | Γ | 0 | 0 | 0.41658 | 0.42007 | 0.42889 |
| ZB | ZnSe | Γ | 0 | 0 | 0.37663 | 0.37930 | 0.39010 |
| WUR | CdS | Γ | 6.47418 | 6.47230 | 0.32580 | 0.32650 | 0.35956 |
| ZB | CdS | Γ | 6.53559 | 6.54140 | 0.39889 | 0.39981 | 0.43550 |
| WUR | CdSe | Γ | 5.88309 | 5.88545 | 0.32035 | 0.32121 | 0.35233 |
| ZB | CdSe | Γ | 5.95534 | 5.96986 | 0.39257 | 0.39352 | 0.42854 |
| WUR | InN | Γ | 9.10558 | 9.06663 | 0.52862 | 0.54518 | 0.59710 |
| ZB | InP | Γ | 4.09751 | 4.09425 | 0.43170 | 0.44293 | 0.47761 |
| ZB | InAs | Γ | 3.92329 | 3.91753 | 0.44275 | 0.45438 | 0.49128 |
| ZB | AlSb | Γ | 0 | 0 | 0.63572 | 0.65734 | 0.70038 |
| ZB | GaSb | Γ | 0 | 0 | 0.56393 | 0.59144 | 0.60167 |
| ZB | InSb | Γ | 0 | 0 | 0.70587 | 0.72975 | 0.78032 |
| ZB | ZnTe | Γ | 0 | 0 | 0.83230 | 0.88844 | 0.93396 |
| ZB | CdTe | Γ | 0 | 0 | 0.80312 | 0.85774 | 0.90484 |
| ZB | HgS | Γ | 6.02816 | 6.03368 | 1.23323 | 1.38897 | 1.55752 |
| ZB | HgSe | Γ | 5.51388 | 5.52433 | 1.21595 | 1.37019 | 1.51837 |
| ZB | HgTe | Γ | 4.24500 | 4.25050 | 1.05571 | 1.19472 | 1.35924 |
| RS | PbS | Γ | 5.21122 | 5.21111 | 2.13329 | 2.51889 | 2.79637 |
| RS | PbSe | Γ | 4.71088 | 4.71237 | 2.00904 | 2.36434 | 2.61193 |
| RS | PbTe | Γ | 4.07581 | 4.08355 | 1.82012 | 2.13599 | 2.34457 |

Table S7: Spin-orbit splittings for the compound semiconductor subset of the band structure benchmark calculated using Benchmark Settings. All values are given in units of eV.

| Prototype | Material | K-Point | SR Energy Wien2k | SR Energy FHI-aims | SO Split APW | SO Split APW+p1/2 | SO Split NAO |
|---|---|---|---|---|---|---|---|
| HCP | Be | N/A | | | | | |
| GRA | C | N/A | | | | | |
| FCC | Ne | Γ | 0 | 0 | 0.10713 | 0.10714 | 0.10317 |
| HCP | Mg | N/A | | | | | |
| FCC | Al | W | -0.83531 | -0.83487 | 0.01669 | 0.01669 | 0.01672 |
| DIA | Si | Γ | 0 | 0 | 0.04762 | 0.04762 | 0.04757 |
| FCC | Ca | N/A | | | | | |
| HCP | Sc | N/A | | | | | |
| HCP | Ti | N/A | | | | | |
| BCC | V | Γ | 0.42232 | 0.42116 | 0.03901 | 0.03901 | 0.03727 |
| BCC | Cr | Γ | -0.84754 | -0.84759 | 0.05334 | 0.05334 | 0.05098 |
| FCC | Mn | Γ | -0.75226 | -0.75518 | 0.07084 | 0.07084 | 0.06792 |
| BCC | Fe | H | 9.59846 | 9.59432 | 0.25340 | 0.25340 | 0.26045 |
| HCP | Co | H | -1.02279 | -1.02378 | 0.11632 | 0.11632 | 0.11255 |
| FCC | Ni | L | -1.88193 | -1.88408 | 0.16400 | 0.16340 | 0.15798 |
| FCC | Cu | L | -3.03742 | -3.04201 | 0.20418 | 0.20419 | 0.19823 |
| HCP | Zn | N/A | | | | | |
| DIA | Ge | Γ | 0 | 0 | 0.28701 | 0.29168 | 0.29811 |
| FCC | Sr | W | 0.59364 | 0.60452 | 0.05073 | 0.05175 | 0.05245 |
| HCP | Y | Γ | 1.73779 | 1.75917 | 0.06756 | 0.06749 | 0.06675 |
| HCP | Zr | Γ | 1.52624 | 1.53410 | 0.11354 | 0.11346 | 0.11174 |
| BCC | Nb | H | 9.11850 | 9.11601 | 0.61245 | 0.61271 | 0.64272 |
| BCC | Mo | H | 9.07448 | 9.07691 | 0.70144 | 0.72290 | 0.73938 |
| HCP | Tc | Γ | -0.11108 | -0.11055 | 0.12306 | 0.12307 | 0.12271 |
| HCP | Ru | Γ | -1.93540 | -1.92825 | 0.29861 | 0.29861 | 0.29669 |
| FCC | Rh | L | -3.15316 | -3.15514 | 0.28231 | 0.28231 | 0.28168 |
| FCC | Pd | X | 0.31998 | 0.30672 | 0.28817 | 0.28817 | 0.28834 |
| FCC | Ag | Γ | -4.75860 | -4.75451 | 0.39208 | 0.39207 | 0.39171 |
| HCP | Cd | N/A | | | | | |
| DIA | Sn | Γ | 2.11807 | 2.11715 | 0.44674 | 0.46096 | 0.49219 |
| FCC | Xe | Γ | 0 | 0 | 1.31738 | 1.33800 | 1.41722 |
| BCC | Ba | H | 4.06142 | 4.09633 | 0.40280 | 0.41991 | 0.48997 |
| HCP | Lu | H | 0.34721 | 0.34983 | 0.26625 | 0.29983 | 0.33629 |
| HCP | Hf | K | -1.81124 | -1.80756 | 0.30523 | 0.32314 | 0.39185 |
| BCC | Ta | P | -1.20022 | -1.20527 | 0.55909 | 0.64460 | 0.72952 |
| BCC | W | H | 5.13960 | 5.13865 | 0.71954 | 0.71777 | 0.74936 |
| HCP | Re | A | -2.36793 | -2.36771 | 0.43285 | 0.43527 | 0.36408 |
| HCP | Os | H | -1.38336 | -1.38196 | 0.65064 | 0.65001 | 0.67135 |
| FCC | Ir | Γ | -3.83656 | -3.84116 | 0.82714 | 0.82666 | 0.85308 |
| FCC | Pt | Γ | -3.77864 | -3.77896 | 0.97698 | 0.97544 | 1.01374 |
| FCC | Au | W | 6.40753 | 6.40521 | 1.06415 | 1.19058 | 1.43020 |
| HCP | Tl | Γ | 7.94648 | 8.05731 | 1.42074 | 1.21881 | 1.17834 |
| FCC | Pb | Γ | 7.38048 | 7.38568 | 2.77384 | 3.32102 | 3.57411 |
| BCC | Bi | Γ | 6.09743 | 6.10457 | 3.46044 | 4.14815 | 4.58284 |
| SCC | Po | Γ | 1.22751 | 1.22973 | 2.82318 | 3.19241 | 3.47393 |

Table S8: Spin-orbit splittings for the elemental materials subset of the band structure benchmark calculated using Benchmark Settings. All values are given in units of eV.

| Prototype | Material | K-Point | SR Energy Wien2k | SR Energy FHI-aims | SO Split APW | SO Split APW+p1/2 | SO Split NAO |
|---|---|---|---|---|---|---|---|
| RS | LiF | Γ | -0.00113 | -0.00108 | 0.06390 | 0.06390 | 0.06098 |
| RS | NaF | Γ | 0 | 0 | 0.06181 | 0.06182 | 0.05884 |
| RS | LiCl | Γ | -0.00319 | -0.00328 | 0.13268 | 0.13272 | 0.13136 |
| RS | NaCl | Γ | 0 | 0 | 0.12703 | 0.12708 | 0.12579 |
| RS | KF | Γ | 0 | 0 | 0.06254 | 0.06256 | 0.05943 |
| RS | KCl | Γ | 0 | 0 | 0.12279 | 0.12284 | 0.12147 |
| RS | LiBr | Γ | -0.00541 | -0.00541 | 0.53553 | 0.53807 | 0.55472 |
| RS | NaBr | Γ | 0 | 0 | 0.51255 | 0.51481 | 0.53256 |
| RS | KBr | Γ | 0 | 0 | 0.48684 | 0.48892 | 0.50505 |
| RS | RbF | Γ | -0.09465 | -0.09259 | 0.08098 | 0.08133 | 0.07846 |
| RS | RbCl | Γ | 0 | 0 | 0.13348 | 0.13375 | 0.13263 |
| RS | RbBr | Γ | 0 | 0 | 0.48924 | 0.49153 | 0.50860 |
| RS | LiI | Γ | -0.01095 | -0.01092 | 1.08052 | 1.10419 | 1.17903 |
| RS | NaI | Γ | 0 | 0 | 1.03575 | 1.05576 | 1.12944 |
| RS | KI | Γ | 0 | 0 | 0.98189 | 1.00058 | 1.06870 |
| RS | RbI | Γ | 0 | 0 | 0.96935 | 0.98715 | 1.05535 |
| RS | CsF | Γ | -4.92078 | -4.94380 | 1.60421 | 1.64733 | 1.74253 |
| CSCL | CsBr | Γ | 0 | 0 | 0.54519 | 0.54966 | 0.57152 |
| CSCL | CsCl | Γ | -5.85268 | -5.85333 | 1.57986 | 1.62345 | 1.71053 |
| RS | CsCl | Γ | -5.66626 | -5.66728 | 1.56249 | 1.59888 | 1.68632 |
| CSCL | CsI | Γ | -7.07602 | -7.07749 | 1.56597 | 1.60992 | 1.69180 |

Table S9: Spin-orbit splittings for the alkali halides subset of the band structure benchmark calculated using Benchmark Settings. All values are given in units of eV.

# 6 Results, Tight Production Settings

Tables S10, S12, and S14 list the spin-orbit splittings calculated by FHI-aims using Tight Production Settings for the PBE and HSE06 functionals. To specify which spin-orbit splitting is being compared across functionals, we indicate the k-point where the spin-orbit splitting occurs alongside the energy eigenvalue of the associated scalar-relativistic eigenstates (i.e. the non-SOC-perturbed eigenvalue) for the PBE and HSE06 functionals. We omit Co and Fe from the comparison of spin-orbit splittings at Tight Production Settings due to difficulty converging the electronic structures on the HSE06 level of theory.

"N/A" denotes either the spin-orbit splittings in the material were too weak to be visually distinguished in the energy range [VBM - 10 eV, VBM + 10 eV] or no unambiguous spin-orbit splitting (i.e. no single scalar-relativistic energy level clearly splitting into two spin-orbit-coupled energy levels) could be visually identified in the energy range. The exceptions are Ge, GaSb, and InSb, where the overall spin-orbit splitting of the highest occupied band at Γ is included in this set despite ambiguity for PBE calculations. For materials whose spin-orbit splittings show subband splitting (see Appendix B), the overall splitting of the energy level is used. The zero of energy is set to the valence band maximum for insulators and the Fermi energy for metals.

Tables S11, S13, and S15 list PBE- and HSE06-calculated fundamental gaps (both on the scalar-relativistic and spin-orbit-coupled levels) as well as changes to fundamental gaps due to spin-orbit coupling $\Delta E_g$ as calculated by FHI-aims using Tight Production Settings. Fundamental gaps were obtained from band structure calculations, as the band structure k-paths were constructed to traverse relevant high-symmetry directions where frontier orbitals are expected to reside. Only hypothetical gapped materials are included in the comparison.

| Prototype | Material | K-Point | SR Energy PBE | SR Energy HSE06 | SO Split PBE | SO Split HSE06 |
|---|---|---|---|---|---|---|
| DIA | C | N/A | | | | |
| RS | MgO | N/A | | | | |
| WUR | AlN | N/A | | | | |
| ZB | AlN | N/A | | | | |
| ZB | SiC | N/A | | | | |
| ZB | BP | N/A | | | | |
| ZB | AlP | Γ | 0 | 0 | 0.05988 | 0.05772 |
| RS | MgS | Γ | 0 | 0 | 0.09306 | 0.09055 |
| WUR | ZnO | H | -4.54949 | -5.71039 | 0.26897 | 0.20755 |
| WUR | ZnS | Γ | 0 | 0 | 0.03121 | 0.03528 |
| ZB | ZnS | Γ | 0 | 0 | 0.05851 | 0.06705 |
| WUR | GaN | Γ | 9.93044 | 11.49491 | 0.22245 | 0.21517 |
| ZB | GaN | N/A | | | | |
| ZB | GaP | Γ | 3.88887 | 4.78003 | 0.16216 | 0.15557 |
| ZB | BAs | Γ | 0 | 0 | 0.20318 | 0.20558 |
| ZB | AlAs | Γ | 0 | 0 | 0.29159 | 0.28247 |
| ZB | GaAs | Γ | 0 | 0 | 0.33028 | 0.32318 |
| RS | MgSe | Γ | 0 | 0 | 0.42559 | 0.41623 |
| ZB | ZnSe | Γ | 0 | 0 | 0.38566 | 0.39070 |
| WUR | CdS | Γ | 6.51215 | 7.66877 | 0.39862 | 0.38264 |
| ZB | CdS | Γ | 6.55849 | 7.72540 | 0.47021 | 0.45187 |
| WUR | CdSe | Γ | 6.05687 | 7.09836 | 0.48245 | 0.47259 |
| ZB | CdSe | Γ | 6.14194 | 7.20041 | 0.57400 | 0.57022 |
| WUR | InN | Γ | 9.16729 | 10.50255 | 0.59138 | 0.54952 |
| ZB | InP | Γ | 4.09715 | 4.92228 | 0.46464 | 0.44018 |
| ZB | InAs | Γ | 3.94196 | 4.67992 | 0.47185 | 0.44692 |
| ZB | AlSb | Γ | 0 | 0 | 0.67924 | 0.65779 |
| ZB | GaSb | Γ | 0 | 0 | 0.72120 | 0.69853 |
| ZB | InSb | Γ | 0 | 0 | 0.76515 | 0.74598 |
| ZB | ZnTe | Γ | 0 | 0 | 0.89776 | 0.88464 |
| ZB | CdTe | Γ | 0 | 0 | 0.87242 | 0.85403 |
| ZB | HgS | Γ | 6.05871 | 7.11499 | 1.71262 | 1.66949 |
| ZB | HgSe | Γ | 5.66240 | 6.59538 | 1.98013 | 1.94315 |
| ZB | HgTe | Γ | 4.35575 | 5.09775 | 1.63647 | 1.59398 |
| RS | PbS | Γ | 5.22266 | 6.00886 | 2.78481 | 2.73074 |
| RS | PbSe | Γ | 4.73487 | 5.45017 | 2.61089 | 2.54566 |
| RS | PbTe | Γ | 4.12909 | 4.75596 | 2.38506 | 2.32680 |

Table S10: Spin-orbit splittings for the compound semiconductors subset of the band structure benchmark calculated using Tight Production Settings. All values are given in units of eV.

| Prototype | Material | Fund. Gap PBE | Fund. Gap HSE06 | Fund. Gap PBE+SOC | Fund. Gap HSE06+SOC | $\Delta E_g$ PBE | $\Delta E_g$ HSE06 |
|---|---|---|---|---|---|---|---|
| DIA | C | 4.14134 | 5.39199 | 4.13710 | 5.38791 | -0.00424 | -0.00408 |
| RS | MgO | 4.66334 | 6.44064 | 4.65164 | 6.42929 | -0.01170 | -0.01135 |
| WUR | AlN | 4.20803 | 5.64467 | 4.20775 | 5.64444 | -0.00028 | -0.00023 |
| ZB | AlN | 3.31294 | 4.63236 | 3.30731 | 4.62691 | -0.00563 | -0.00545 |
| ZB | SiC | 1.37116 | 2.35182 | 1.36712 | 2.34780 | -0.00404 | -0.00402 |
| ZB | BP | 1.24188 | 2.03224 | 1.22836 | 2.01863 | -0.01352 | -0.01361 |
| ZB | AlP | 1.58205 | 2.32357 | 1.56195 | 2.30420 | -0.02010 | -0.01937 |
| RS | MgS | 2.77819 | 3.84373 | 2.74700 | 3.81338 | -0.03119 | -0.03035 |
| WUR | ZnO | 0.81010 | 2.44768 | 0.79040 | 2.43557 | -0.01970 | -0.01211 |
| WUR | ZnS | 2.15885 | 3.29186 | 2.13786 | 3.26848 | -0.02099 | -0.02338 |
| ZB | ZnS | 2.10854 | 3.24137 | 2.08784 | 3.21819 | -0.02070 | -0.02318 |
| WUR | GaN | 1.91941 | 3.16801 | 1.91673 | 3.16453 | -0.00268 | -0.00348 |
| ZB | GaN | 1.67628 | 2.90351 | 1.67251 | 2.89903 | -0.00377 | -0.00448 |
| ZB | GaP | 1.59959 | 2.28267 | 1.57257 | 2.25562 | -0.02702 | -0.02705 |
| ZB | BAs | 1.18760 | 1.88615 | 1.12065 | 1.81758 | -0.06695 | -0.06857 |
| ZB | AlAs | 1.44302 | 2.10852 | 1.34187 | 2.01060 | -0.10115 | -0.09792 |
| ZB | GaAs | 0.53041 | 1.32227 | 0.41542 | 1.20995 | -0.11499 | -0.11232 |
| RS | MgSe | 1.78414 | 2.66284 | 1.63622 | 2.51829 | -0.14792 | -0.14455 |
| ZB | ZnSe | 1.29961 | 2.29503 | 1.16387 | 2.15841 | -0.13574 | -0.13662 |
| WUR | CdS | 1.17665 | 2.10581 | 1.15826 | 2.08590 | -0.01839 | -0.01991 |
| ZB | CdS | 1.15196 | 2.07842 | 1.13371 | 2.05864 | -0.01825 | -0.01978 |
| WUR | CdSe | 0.67493 | 1.50336 | 0.54432 | 1.37319 | -0.13061 | -0.13017 |
| ZB | CdSe | 0.65644 | 1.48351 | 0.52513 | 1.35298 | -0.13131 | -0.13053 |
| WUR | InN | 0 | 0.65752 | 0 | 0.65440 | 0 | -0.00312 |
| ZB | InP | 0.71223 | 1.43839 | 0.67649 | 1.40153 | -0.03574 | -0.03686 |
| ZB | InAs | 0 | 0.41883 | 0 | 0.29637 | 0 | -0.12246 |
| ZB | AlSb | 1.20389 | 1.74504 | 0.94946 | 1.49900 | -0.25443 | -0.24604 |
| ZB | GaSb | 0.12698 | 0.83469 | 0 | 0.57371 | -0.12686 | -0.26098 |
| ZB | InSb | 0 | 0.43095 | 0 | 0.14773 | 0 | -0.28322 |
| ZB | ZnTe | 1.25344 | 2.15402 | 0.90819 | 1.81620 | -0.34525 | -0.33782 |
| ZB | CdTe | 0.78659 | 1.54898 | 0.44776 | 1.21917 | -0.33883 | -0.32981 |
| ZB | HgS | 0 | 0.34991 | 0.03755 | 0.25101 | +0.03755 | -0.09890 |
| RS | PbS | 0.36994 | 0.77573 | 0.11255 | 0.55106 | -0.25739 | -0.22467 |
| RS | PbSe | 0.30717 | 0.67344 | 0.00596 | 0.40301 | -0.30121 | -0.27043 |
| RS | PbTe | 0.73470 | 1.09110 | 0.08923 | 0.46479 | -0.64547 | -0.62631 |

Table S11: Fundamental gaps, without and with spin-orbit coupling, and changes in fundamental gaps due to spin-orbit coupling for the compound semiconductors subset of the band structure benchmark calculated using Tight Production Settings. All values are given in units of eV.

| Prototype | Material | K-Point | SR Energy PBE | SR Energy HSE06 | SO Split PBE | SO Split HSE06 |
|---|---|---|---|---|---|---|
| HCP | Be | N/A | | | | |
| GRA | C | N/A | | | | |
| FCC | Ne | Γ | 0 | 0 | 0.10306 | 0.10229 |
| HCP | Mg | N/A | | | | |
| FCC | Al | W | -0.83558 | -0.99022 | 0.01670 | 0.01574 |
| DIA | Si | Γ | 0 | 0 | 0.04593 | 0.04492 |
| FCC | Ca | N/A | | | | |
| HCP | Sc | N/A | | | | |
| HCP | Ti | N/A | | | | |
| BCC | V | Γ | 0.41314 | 0.78755 | 0.03697 | 0.03599 |
| BCC | Cr | Γ | -0.82724 | -1.31666 | 0.05065 | 0.04947 |
| FCC | Mn | Γ | -0.77643 | -1.67090 | 0.06728 | 0.06484 |
| FCC | Ni | L | -1.88823 | -2.68161 | 0.15775 | 0.13837 |
| FCC | Cu | L | -2.93869 | -4.19897 | 0.19799 | 0.19226 |
| HCP | Zn | N/A | | | | |
| DIA | Ge | Γ | 0 | 0 | 0.28873 | 0.28430 |
| FCC | Sr | W | 0.61915 | 0.83772 | 0.05743 | 0.06321 |
| HCP | Y | Γ | 1.73635 | 2.32100 | 0.06625 | 0.06230 |
| HCP | Zr | Γ | 1.52162 | 2.03780 | 0.11110 | 0.10467 |
| BCC | Nb | H | 9.16606 | 9.94267 | 0.68048 | 0.66803 |
| BCC | Mo | H | 9.17671 | 9.79572 | 0.78037 | 0.76895 |
| HCP | Tc | Γ | -0.11665 | -0.09156 | 0.12048 | 0.11790 |
| HCP | Ru | Γ | -1.89960 | -2.39512 | 0.29273 | 0.28618 |
| FCC | Rh | L | -3.09815 | -3.85843 | 0.27859 | 0.26218 |
| FCC | Pd | X | 0.29643 | 0.42674 | 0.28786 | 0.25788 |
| FCC | Ag | Γ | -4.76648 | -6.00401 | 0.38840 | 0.38420 |
| HCP | Cd | N/A | | | | |
| DIA | Sn | Γ | 2.17880 | 2.64030 | 0.50875 | 0.49896 |
| FCC | Xe | Γ | 0 | 0 | 1.39861 | 1.37858 |
| BCC | Ba | H | 4.19041 | 4.64181 | 0.57378 | 0.66421 |
| HCP | Lu | H | 0.34564 | 0.33299 | 0.34994 | 0.38087 |
| HCP | Hf | K | -1.79720 | -2.31985 | 0.38272 | 0.41106 |
| BCC | Ta | P | -1.18011 | -1.55592 | 0.71421 | 0.76557 |
| BCC | W | H | 5.26913 | 5.93609 | 0.73591 | 0.73625 |
| HCP | Re | A | -2.32665 | -2.76990 | 0.34737 | 0.45914 |
| HCP | Os | H | -1.44453 | -1.68431 | 0.65931 | 0.64588 |
| FCC | Ir | Γ | -3.91697 | -4.48429 | 0.84088 | 0.83156 |
| FCC | Pt | Γ | -3.80654 | -4.37808 | 0.99810 | 0.99320 |
| FCC | Au | W | 6.57406 | 7.38788 | 1.47040 | 1.49845 |
| HCP | Tl | Γ | 8.13598 | 8.78148 | 1.29131 | 1.48045 |
| FCC | Pb | Γ | 7.60057 | 8.37095 | 3.97824 | 3.85776 |
| BCC | Bi | Γ | 6.09255 | 6.76602 | 4.84683 | 4.86949 |
| SCC | Po | Γ | 1.23112 | 1.39008 | 3.47932 | 3.40531 |

Table S12: Spin-orbit splittings for the elemental materials subset of the band structure benchmark calculated using Tight Production Settings. All values are given in units of eV.

| Prototype | Material | Fund. Gap PBE | Fund. Gap HSE06 | Fund. Gap PBE+SOC | Fund. Gap HSE06+SOC | $\Delta E_g$ PBE | $\Delta E_g$ HSE06 |
|---|---|---|---|---|---|---|---|
| FCC | Ne | 11.63090 | 14.39768 | 11.59655 | 14.36359 | -0.03435 | -0.03409 |
| DIA | Si | 0.58506 | 1.18516 | 0.56964 | 1.17008 | -0.01542 | -0.01508 |
| DIA | Ge | 0.04877 | 0.77516 | 0 | 0.67654 | -0.04877 | -0.09862 |
| FCC | Xe | 6.26445 | 7.42879 | 5.72377 | 6.89763 | -0.54068 | -0.53116 |

Table S13: Fundamental gaps, without and with spin-orbit coupling, and changes in fundamental gaps due to spin-orbit coupling for the elemental materials subset of the band structure benchmark calculated using Tight Production Settings. All values are given in units of eV.

| Prototype | Material | K-Point | SR Energy PBE | SR Energy HSE06 | SO Split PBE | SO Split HSE06 |
|---|---|---|---|---|---|---|
| RS | LiF | Γ | -0.00108 | -0.00058 | 0.06084 | 0.06015 |
| RS | NaF | Γ | 0 | 0 | 0.05842 | 0.05749 |
| RS | LiCl | Γ | -0.00328 | -0.00230 | 0.13108 | 0.12847 |
| RS | NaCl | Γ | 0 | 0 | 0.12528 | 0.12261 |
| RS | KF | Γ | 0 | 0 | 0.05942 | 0.05896 |
| RS | KCl | Γ | 0 | 0 | 0.12111 | 0.11866 |
| RS | LiBr | Γ | -0.00550 | -0.00437 | 0.54576 | 0.53548 |
| RS | NaBr | Γ | 0 | 0 | 0.52157 | 0.51097 |
| RS | KBr | Γ | 0 | 0 | 0.49478 | 0.48478 |
| RS | RbF | Γ | -0.09223 | -0.14110 | 0.07757 | 0.08097 |
| RS | RbCl | Γ | 0 | 0 | 0.13103 | 0.12949 |
| RS | RbBr | Γ | 0 | 0 | 0.49502 | 0.48601 |
| RS | LiI | Γ | -0.01119 | -0.00920 | 1.14235 | 1.12591 |
| RS | NaI | Γ | 0 | 0 | 1.09513 | 1.07717 |
| RS | KI | Γ | 0 | 0 | 1.03627 | 1.01937 |
| RS | RbI | Γ | 0 | 0 | 1.01869 | 1.00295 |
| RS | CsF | Γ | -4.97487 | -4.63091 | 1.70358 | 1.65233 |
| CSCL | CsBr | Γ | 0 | 0 | 0.56039 | 0.55476 |
| CSCL | CsCl | Γ | -5.89508 | -6.02541 | 1.67931 | 1.65310 |
| RS | CsCl | Γ | -5.70761 | -5.82424 | 1.65985 | 1.63719 |
| CSCL | CsI | Γ | -7.10572 | -7.52175 | 1.67121 | 1.65202 |

Table S14: Spin-orbit splittings for the alkali halides subset of the band structure benchmark calculated using Tight Production Settings. All values are given in units of eV.

| Prototype | Material | Fund. Gap PBE | Fund. Gap HSE06 | Fund. Gap PBE+SOC | Fund. Gap HSE06+SOC | $\Delta E_g$ PBE | $\Delta E_g$ HSE06 |
|---|---|---|---|---|---|---|---|
| RS | LiF | 9.15430 | 11.41078 | 9.13507 | 11.39121 | -0.01923 | -0.01957 |
| RS | NaF | 6.33361 | 8.52023 | 6.31414 | 8.50106 | -0.01947 | -0.01917 |
| RS | LiCl | 6.32817 | 7.65985 | 6.28749 | 7.61909 | -0.04068 | -0.04076 |
| RS | NaCl | 5.08753 | 6.41425 | 5.04552 | 6.37316 | -0.04201 | -0.04109 |
| RS | KF | 6.13611 | 8.17035 | 6.11627 | 8.15067 | -0.01984 | -0.01968 |
| RS | KCl | 5.16432 | 6.46532 | 5.12370 | 6.42553 | -0.04062 | -0.03979 |
| RS | LiBr | 4.93003 | 6.07768 | 4.74543 | 5.89569 | -0.18460 | -0.18199 |
| RS | NaBr | 4.13834 | 5.27209 | 3.95648 | 5.09411 | -0.18186 | -0.17798 |
| RS | KBr | 4.41090 | 5.53364 | 4.23816 | 5.36460 | -0.17274 | -0.16904 |
| RS | RbF | 5.68226 | 7.61927 | 5.67628 | 7.61250 | -0.00598 | -0.00677 |
| RS | RbCl | 4.97209 | 6.26505 | 4.92755 | 6.22104 | -0.04454 | -0.04401 |
| RS | RbBr | 4.34798 | 5.47209 | 4.17483 | 5.30233 | -0.17315 | -0.16976 |
| RS | LiI | 4.27607 | 5.25320 | 3.85052 | 4.83295 | -0.42555 | -0.42025 |
| RS | NaI | 3.62727 | 4.57651 | 3.20729 | 4.16467 | -0.41998 | -0.41184 |
| RS | KI | 3.94196 | 4.87936 | 3.54342 | 4.48860 | -0.39854 | -0.39076 |
| RS | RbI | 3.88380 | 4.82545 | 3.49187 | 4.44089 | -0.39193 | -0.38456 |
| RS | CsF | 5.43391 | 7.23338 | 5.38751 | 7.17620 | -0.04640 | -0.05718 |
| CSCL | CsBr | 4.52875 | 5.63066 | 4.32653 | 5.43050 | -0.20222 | -0.20016 |
| CSCL | CsCl | 5.26488 | 6.52957 | 5.18768 | 6.45019 | -0.07720 | -0.07938 |
| RS | CsCl | 4.87689 | 6.12226 | 4.79110 | 6.03416 | -0.08579 | -0.08810 |
| CSCL | CsI | 3.88761 | 4.80882 | 3.56247 | 4.49788 | -0.32514 | -0.31094 |

Table S15: Fundamental gaps, without and with spin-orbit coupling, and changes in fundamental gaps due to spin-orbit coupling for the alkali halides subset of the band structure benchmark calculated using Tight Production Settings. All values are given in units of eV.

# A Comparison of Valence and Semi-Core Energies for Free Cd and Hg Atoms

In this Appendix, we list the computational settings used for the comparison of valence and semi-core energy eigenvalues of free Hg and Cd atoms with different relativistic approximations for FHI-aims (Table S16), Wien2k (Table S17), and dftatom (Table S18). Energy eigenvalues are listed in Table S19. In each calculation, the HOMO (5s orbital for Cd, 6s orbital for Hg) has been set to the zero of energy. All calculations used Perdew and Wang's RPA parameterization of the LDA functional [16]. For Wien2k, a 10 Å unit cell and a gamma-point-only s.c.f. k-grid was used.

| Atom | Integration Settings | Basis Set |
|---|---|---|
| Cd | Really Tight | Tier 2 |
| Hg | Really Tight | Tier 2 |

Table S16: Settings used for FHI-aims for comparison of free Cd and Hg atom across across codes, basis sets, and relativistic treatments.

| Atom | $R_{MT}$ | $RK_{max}$ |
|---|---|---|
| Cd | 1.60 | 10.00 |
| Hg | 2.26 | 12.00 |

Table S17: Settings used for Wien2k for comparison of free Cd and Hg atom across codes, basis sets, and relativistic treatments. $R_{MT}$ for Hg has been increased relative to Benchmark Settings (see Table S2).

| Atom | Relativistic Handling | Number of Points |
|---|---|---|
| Cd | NR | 11029 |
| Hg | NR | 15641 |
| Cd | Dirac | 11272 |
| Hg | Dirac | 16463 |

Table S18: Settings used for dftatom for comparison of free Cd and Hg atom across codes, basis sets, and relativistic treatments. "NR" denotes non-relativistic calculations.

| Orbital | NAO | APW | APW+$p^{1/2}$ | dftatom |
|---|---|---|---|---|
| Cd 4d (NR) | -7.236 | -7.253 | | -7.242 |
| Cd 4d (SR) | -5.949 | -5.953 | | |
| Cd $4d_{5/2}$ | -5.669 | -5.683 | -5.682 | -5.664 |
| Cd $4d_{3/2}$ | -6.368 | -6.383 | -6.382 | -6.366 |
| Spin-Orbit Splitting | 0.699 | 0.700 | 0.700 | 0.702 |
| Hg 5d (NR) | -6.723 | -6.736 | | -6.728 |
| Hg 5d (SR) | -2.958 | -2.952 | | |
| Hg $5d_{5/2}$ | -2.178 | -2.282 | -2.231 | -2.226 |
| Hg $5d_{3/2}$ | -4.075 | -4.117 | -4.056 | -4.076 |
| Spin-Orbit Splitting | 1.897 | 1.835 | 1.816 | 1.850 |
| Hg 5p (NR) | -55.958 | -55.979 | | -55.964 |
| Hg 5p (SR) | -59.552 | -59.522 | | |
| Hg $5p_{3/2}$ | -51.284 | -54.510 | -54.645 | -54.659 |
| Hg $5p_{1/2}$ | -71.363 | -70.568 | -73.098 | -73.145 |
| Spin-Orbit Splitting | 20.079 | 16.058 | 18.453 | 18.486 |

Table S19: Energy levels for select orbitals of free Cd and Hg atoms, calculated with the Perdew and Wang's RPA parameterization of the LDA functional, for various relativistic approximations and various computational methods (described in main text). "NR" denotes non-relativistic calculations and "SR" denotes scalar-relativistic calculations. All values are given in units of eV.

# B Dependence of Spin-Orbit Splittings Calculated by FHI-aims on Basis Set Size and Number of Calculated Eigenstates

In this final Appendix, we briefly quantify the dependence of spin-orbit splittings on two computational parameters entering into second-variational spin-orbit coupling in FHI-aims: the basis set size and the number of empty eigenstates (per atom) calculated. The latter is formally important for second-variational SOC as this level of theory uses the space of calculated eigenstates as a basis set, suggesting a secondary basis set convergence criteria is needed.

We also consider the phenomena of "sub-banding" observed in FHI-aims' second-variational spin-orbit coupling, in which a (formally) degenerate SOC-perturbed band will have a slight splitting into several subbands nearly-but-not-quite degenerate in energy. In most cases, this subbanding is on the order of 0.00001 eV. (We note that in every band structure examined by the authors, Kramer's theorem continues to hold: that is, every sub-band occurring at time-inversion-symmetric k-points continue to have an even degeneracy number.)

Shown in Tables S20, S21, and S22 are the spin-orbit splittings for materials with a maximum atomic number $Z_{max} \geq 48$ (Cd) where the basis set size is varied from Tight, Tier 2, to Tier 3, respectively. CdSe (WUR) and ZnTe are omitted from this table, as they were late additions to the benchmark set. We also consider two sets of calculations with differing number of calculated eigenstates entering into second-variational spin-orbit coupling: one set of calculations with the default number of empty states calculated by FHI-aims (see main text for more information) and the other set with a fixed value of 50 empty states per atom, greatly exceeding the default values. For this comparison, tight integration settings were used.

We do find evidence for a basis set dependence going from Tight to Tier 2 basis sets for spin-orbit splittings occurring in high-lying conduction states, but no clear evidence for a basis set dependence for spin-orbit splittings occurring in valence and low-lying conductions states. It should be emphasized that we find spin-orbit splittings calculated using Tier 2 and Tier 3 basis sets are similar for the heaviest materials in the band structure benchmark. The differences between FHI-aims- and Wien2k-calculated values for Benchmark Settings are not attributable to the size of the Tier 2 basis set but rather the fundamentally scalar-relativistic nature of the basis set.

We find a weak dependence for the magnitude of spin-orbit splittings as a function of the number of states used. Notably, we find a trend that spin-orbit splittings for materials with $Z \leq 78$ (Pt) weakly increase when the number of states is increased. The weakness of this trend is expected, as $v_{SOC}$ has appreciable strength only in the nuclear region, suggesting relatively weak coupling between states well-removed in energy. This trend is reversed for materials with $Z \geq 79$ (Au), where a decrease in the magnitude of spin-orbit splitting is observed.

| Prototype | Material | K-Point | SR Energy | SO Splitting, Default Number Empty States | SO Splitting, 50 Empty States per Atom |
|---|---|---|---|---|---|
| HCP | Cd | N/A | | | |
| WUR | CdS | Γ | 6.51167 | 0.39873 (0) | 0.40250 (0) |
| ZB | CdS | Γ | 6.55790 | 0.46606 (0.00109) | 0.47042 (0.00002) |
| ZB | CdSe | Γ | 6.14200 | 0.57449 (0.00008) | 0.57935 (0.00007) |
| WUR | InN | Γ | 9.16539 | 0.59131 (0) | 0.60835 (0) |
| ZB | InP | Γ | 4.09783 | 0.46474 (0.00060) | 0.47627 (0.00003) |
| ZB | InAs | Γ | 3.92222 | 0.47210 (0.00016) | 0.48349 (0.00018) |
| DIA | Sn | Γ | 2.17842 | 0.50878 (0.00016) | 0.51508 (0.00017) |
| ZB | AlSb | Γ | 0 | 0.67937 (0.00059) | 0.68970 (0.00022) |
| ZB | GaSb | Γ | 0 | 0.72129 (0.14255*) | 0.73015 (0.13778*) |
| ZB | InSb | Γ | 0 | 0.76504 (0.29374*) | 0.77334 (0.30708*) |
| ZB | CdTe | Γ | 0 | 0.87235 (0.00004) | 0.89141 (0.00003) |
| RS | LiI | Γ | -0.01105 | 1.14222 (0.00001) | 1.15450 (0.00001) |
| RS | NaI | Γ | 0 | 1.09590 (0.00001) | 1.10896 (0.00001) |
| RS | KI | Γ | 0 | 1.03586 (0.00001) | 1.04973 (0) |
| RS | RbI | Γ | 0 | 1.01845 (0) | 1.03218 (0) |
| FCC | Xe | Γ | 0 | 1.39868 (0) | 1.41466 (0) |
| RS | CsF | Γ | -4.97387 | 1.70291 (0.00032) | 1.72994 (0.00002) |
| CSCL | CsBr | Γ | 0 | 0.56058 (0.00003) | 0.56416 (0) |
| CSCL | CsCl | Γ | -5.88591 | 1.67906 (0.00324) | 1.68849 (0.00001) |
| RS | CsCl | Γ | -5.69979 | 1.65927 (0) | 1.67670 (0) |
| CSCL | CsI | Γ | -7.10240 | 1.67114 (0) | 1.67722 (0.00001) |
| BCC | Ba | H | 4.11491 | 0.54913 (0) | 0.55566 (0.00002) |
| HCP | Lu | H | 0.31946 | 0.34951 (0.00038) | 0.35569 (0.00236) |
| BCC | Ta | P | -1.20350 | 0.71067 (0.00002) | 0.71297 (0.00118) |
| BCC | W | H | 5.13554 | 0.73583 (0.00002) | 0.73514 (0.00002) |
| HCP | Re | A | -2.36804 | 0.34881 (0.00141) | 0.36045 (0.00036) |
| HCP | Os | H | -1.38155 | 0.65890 (0.00019) | 0.65969 (0.00017) |
| FCC | Ir | Γ | -3.84548 | 0.84025 (0.00006) | 0.85114 (0.00008) |
| FCC | Pt | Γ | -3.73981 | 0.99894 (0.00007) | 1.01083 (0.00008) |
| FCC | Au | W | 6.40489 | 1.47042 (0.00006) | 1.46674 (0.00008) |
| ZB | HgS | Γ | 6.05839 | 1.72144 (0.01736) | 1.71228 (0.00002) |
| ZB | HgSe | Γ | 5.66288 | 1.98066 (0.00008) | 1.98023 (0.00007) |
| ZB | HgTe | Γ | 4.35591 | 1.64876 (0.02672) | 1.63611 (0) |
| HCP | Tl | Γ | 8.13699 | 1.10081 (0) | 1.29083 (0) |
| FCC | Pb | Γ | 7.53677 | 3.9223 (0.02760) | 3.9783 (0.18182) |
| RS | PbS | Γ | 5.22285 | 2.81063 (0.00336) | 2.78551 (0.00004) |
| RS | PbSe | Γ | 4.73519 | 2.63393 (0.00003) | 2.61091 (0.00005) |
| RS | PbTe | Γ | 4.12957 | 2.40323 (0.01677) | 2.38586 (0.00002) |
| BCC | Bi | Γ | 6.15211 | 4.84047 (0.00003) | 4.84668 (0.04583) |
| SCC | Po | Γ | 1.32297 | 3.52504 (0.10457) | 3.47878 (0) |

Table S20: Dependence of spin-orbit splittings on empty_states when using the "tight" basis set in FHI-aims for materials containing species with $Z \geq 48$ (Cd). The numbers in parentheses correspond to the sub-band splitting. *For GaSb and InSb, the subbanding arises from the intermixing of bands due to the unphysically low band gap predicted by the PBE functional and not the choice of basis set or number of empty states included.

| Prototype | Material | K-Point | SR Energy | SO Splitting Default Number Empty States | SO Splitting 50 Empty States per Atom |
|---|---|---|---|---|---|
| HCP | Cd | N/A | | | |
| WUR | CdS | Γ | 6.47188 | 0.34696 (0) | 0.35291 (0) |
| ZB | CdS | Γ | 6.54085 | 0.42190 (0.00052) | 0.42861 (0.00006) |
| ZB | CdSe | Γ | 5.97009 | 0.41488 (0.00012) | 0.42126 (0.00011) |
| WUR | InN | Γ | 9.10281 | 0.57929 (0) | 0.58902 (0) |
| ZB | InP | Γ | 4.09357 | 0.46470 (0.00001) | 0.47073 (0.00001) |
| ZB | InAs | Γ | 3.91718 | 0.47885 (0.00005) | 0.48487 (0.00004) |
| DIA | Sn | Γ | 2.15237 | 0.47215 (0.00004) | 0.48019 (0.00004) |
| ZB | AlSb | Γ | 0 | 0.67932 (0.00049) | 0.68732 (0.00019) |
| ZB | GaSb | Γ | 0 | 0.72561 (0.15528*) | 0.73378 (0.15081*) |
| ZB | InSb | Γ | 0 | 0.75908 (0.27482*) | 0.76688 (0.28734*) |
| ZB | CdTe | Γ | 0 | 0.87733 (0.00006) | 0.89081 (0.00007) |
| RS | LiI | Γ | -0.01089 | 1.14218 (0.00001) | 1.15426 (0.00065) |
| RS | NaI | Γ | 0 | 1.09597 (0.00001) | 1.10673 (0.00001) |
| RS | KI | Γ | 0 | 1.03765 (0) | 1.04767 (0.00063) |
| RS | RbI | Γ | 0 | 1.02556 (0) | 1.03628 (0) |
| FCC | Xe | Γ | 0 | 1.39951 (0) | 1.41566 (0) |
| RS | CsF | Γ | -4.94685 | 1.70415 (0.00002) | 1.73085 (0) |
| CSCL | CsBr | Γ | 0 | 0.56363 (0.00002) | 0.56687 (0.00001) |
| CSCL | CsCl | Γ | -5.85364 | 1.68054 (0) | 1.70604 (0.00001) |
| RS | CsCl | Γ | -5.66649 | 1.65969 (0.00006) | 1.67960 (0) |
| CSCL | CsI | Γ | -7.07746 | 1.67109 (0) | 1.68824 (0) |
| BCC | Ba | H | 4.09677 | 0.48060 (0) | 0.48868 (0.00001) |
| HCP | Lu | H | 0.34997 | 0.32281 (0.00031) | 0.33087 (0.00033) |
| BCC | Ta | P | -1.20374 | 0.70815 (0.00001) | 0.71200 (0.00455) |
| BCC | W | H | 5.14145 | 0.74821 (0.00007) | 0.74614 (0.00008) |
| HCP | Re | A | -2.36606 | 0.34580 (0.00153) | 0.35951 (0.00114) |
| HCP | Os | H | -1.38514 | 0.66724 (0.00021) | 0.66819 (0.00019) |
| FCC | Ir | Γ | -3.84186 | 0.84613 (0.00002) | 0.85439 (0.00059) |
| FCC | Pt | Γ | -3.75751 | 1.00289 (0.00007) | 1.01244 (0.00011) |
| FCC | Au | W | 6.40530 | 1.44808 (0.00006) | 1.42723 (0.00006) |
| ZB | HgS | Γ | 6.03345 | 1.50851 (0.01117) | 1.50267 (0.00010) |
| ZB | HgSe | Γ | 5.52478 | 1.47240 (0.00010) | 1.47282 (0.00010) |
| ZB | HgTe | Γ | 4.25049 | 1.32296 (0.01511) | 1.31297 (0.00003) |
| HCP | Tl | Γ | 8.05794 | 1.12191 (0) | 1.24489 (0) |
| FCC | Pb | Γ | 7.36392 | 3.59277 (0.08395) | 3.53100 (0.00002) |
| RS | PbS | Γ | 5.21108 | 2.75336 (0.00001) | 2.78873 (0) |
| RS | PbSe | Γ | 4.71262 | 2.63202 (0.00001) | 2.60272 (0.00001) |
| RS | PbTe | Γ | 4.08368 | 2.3605 (0.02493) | 2.32170 (0) |
| BCC | Bi | Γ | 6.15105 | 4.59146 (0.00003) | 4.56261 (0.00004) |
| SCC | Po | Γ | 1.31487 | 3.51212 (0.10618) | 3.4542 (0.02251) |

Table S21: Dependence of spin-orbit splittings on empty_states when using the "Tier 2" basis set in FHI-aims for materials containing species with Z≥48 (Cd). The numbers in parentheses correspond to the magnitude of the sub-band splitting. *For GaSb and InSb, the subbanding arises from the intermixing of bands due to the unphysically low band gap predicted by the PBE functional and not the choice of basis set used.

| Prototype | Material | K-Point | SR Energy | SO Splitting<br>Default Number<br>Empty States | SO Splitting<br>50 Empty States<br>per Atom |
|---|---|---|---|---|---|
| HCP | Tl | Γ | 8.04199 | 1.13931 (0.00000) | 1.23207 (0.00000) |
| FCC | Pb | Γ | 7.36401 | 3.58447 (0.08332) | 3.52334 (0.00001) |
| RS | PbTe | Γ | 4.07799 | 2.31201 (0.02580) | 2.30390 (0) |
| BCC | Bi | Γ | 6.14925 | 4.60265 (0.00002) | 4.57503 (0.00003) |
| SCC | Po | Γ | 1.31059 | 3.52582 (0.09774) | 3.46275 (0) |

Table S22: Dependence of spin-orbit splittings on empty_states when using the "Tier 3" basis set in FHI-aims for a select set of materials. The numbers in parentheses correspond to the magnitude of the sub-band splitting.

| Prototype | Material | K-Point | SR Energy | SO Splitting<br>Default Number<br>Empty States | SO Splitting<br>50 Empty States<br>per Atom |
|---|---|---|---|---|---|
| ZB | HgS | Γ | 6.03344 | 1.51090 (0.01116) | 1.50472 (0.00010) |
| ZB | HgSe | Γ | 5.53340 | 1.45585 (0.00016) | 1.45636 (0.00015) |
| ZB | HgTe | Γ | 4.27933 | 1.28665 (0.01778) | 1.27653 (0.00004) |
| RS | PbS | Γ | 5.21243 | 2.75001 (0.00001) | 2.78455 (0) |
| RS | PbSe | Γ | 4.71399 | 2.63160 (0.00001) | 2.60199 (0) |
| RS | PbTe | Γ | 4.09314 | 2.37639 (0.02248) | 2.33643 (0.00001) |

Table S23: Dependence of spin-orbit splittings on empty_states when using mixed basis sets in FHI-aims ("Tier 2" basis set for Hg and Pb and the "tight" basis set for chalcogenides). The numbers in parentheses correspond to the magnitude of the sub-band splitting.

# C Band Structure Comparison for Spin-Polarized FCC Ni

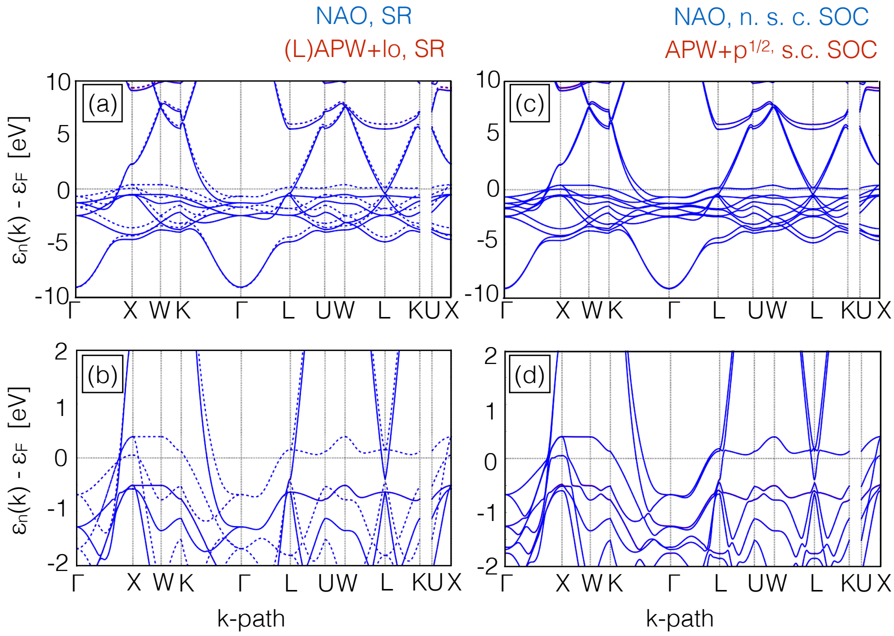


Figure S1: A comparison of PBE band structures of FCC Ni calculated using FHI-aims (tier 2) and WIEN2k ($RK_{max} = 10$) on (a) spin-polarized SR and (c) SOC levels of theory. Close-ups near the Fermi level for spin-polarized SR and SOC levels of theory are shown in (b) and (d) respectively. Spin-up SR levels are denoted by solid lines, and spin-down SR levels are denoted by dashed lines. No such distinction is made on the SOC level, as SOC formally destroys the goodness of the spin quantum number. Benchmark Settings and the experimental lattice parameter of 3.5232 Å is used.

Scalar-relativistic calculations were performed without spin-polarization in this work, but several of the materials in the benchmark set are experimentally spin-polarized. To verify that the trends reported in this work extend to systems that are spin-polarized on the scalar-relativistic level, we provide a comparison in Figure S1 of computed band structures for FCC Ni on the spin-polarized scalar-relativistic and subsequent spin-orbit-coupled levels of theory. Results are consistent with the trends observed in the main text. Excellent agreement in valence and low-lying conduction energy levels is observed between FHI-aims and WIEN2k on the spin-polarized scalar-relativistic level of theory. NAO n.s.c. SOC similarly reproduces the spin-orbit-coupled band structure predicted by APW+$p^{1/2}$ s.c. SOC, notably in the [-2 eV, -1.5 eV] energy range where scalar-relativistic bands from differing spin channels intermix. Weak spin-orbit splittings are observed due to the low atomic number ($Z = 29$) of this material.

# References


[1] The NOMAD Laboratory: A European Centre of Excellence, accessed April 26, 2017. http://nomad-repository.eu.

[2] S. Adachi. *Handbook on physical properties of semiconductors.* Kluwer Academic Publishers, 2004.

[3] P. Blaha, K. Schwarz, G. K. H. Madsen, D. Kvasnicka, and J. Luitz. *WIEN2k, An Augmented Plane Wave + Local Orbitals Program for Calculating Crystal Properties (Karlheinz Schwarz, Techn. Universitat Wien, Austria)*, 2001. ISBN 3-9501031-1-2.

[4] V. Blum, R. Gehrke, F. Hanke, P. Havu, V. Havu, X. Ren, K. Reuter, and M. Scheffler. Ab initio molecular simulations with numeric atom-centered orbitals. *Comp. Phys. Comm.*, 180:2175–2196, 2009.

[5] J. Heyd, G. E. Scuseria, and M. Ernzerhof. Hybrid functionals based on a screened Coulomb potential. *J. Chem. Phys.*, 118:8207–8215, 2003.

[6] J. Heyd, G. E. Scuseria, and M. Ernzerhof. Erratum: "Hybrid functionals based on a screened Coulomb potential" [J. Chem. Phys. 118, 8207 (2003)]. *J. Chem. Phys.*, 124:219906, 2006.

[7] W. P. Huhn and V. Blum, 2017. doi:10.17172/NOMAD/2017.04.27-1.

[8] W. P. Huhn and V. Blum, 2017. doi:10.17172/NOMAD/2017.04.27-2.

[9] W. P. Huhn and V. Blum, 2017. doi:10.17172/NOMAD/2017.04.27-3.

[10] A. V. Krukau, O. A. Vydrov, A. F. Izmaylov, and G. E. Scuseria. Influence of the exchange screening parameter on the performance of screened hybrid functionals. *J. Chem. Phys.*, 125:224106, 2006.

[11] K. Lejaeghere, V. van Speybroeck, G. van Oost, and S. Cottenier. Error estimates for solid-state density-functional theory predictions: an overview by means of the ground-state elemental crystals. *Crit. Rev. Solid State Mater. Sci.*, 39(1):1–24, 2014.

[12] Kurt Lejaeghere, Gustav Bihlmayer, Torbjörn Björkman, Peter Blaha, Stefan Blügel, Volker Blum, Damien Caliste, Ivano E Castelli, Stewart J Clark, Andrea Dal Corso, et al. Reproducibility in density functional theory calculations of solids. *Science*, 351(6280):aad3000, 2016.

[13] H. J. Monkhorst and J. D. Pack. Special points for Brillouin-zone integrations. *Phys. Rev. B*, 13(12):5188–5192, June 1976.

[14] R. J. Nelmes and M. I. McMahon. Structural transitions in the Group IV, III-V, and II-VI semiconductors under pressure. In *Semiconductors and Semimetals*, volume 54, pages 145–246. Academic Press, 1998.

[15] J. P. Perdew, K. Burke, and M. Ernzerhof. Generalized Gradient Approximation made simple. *Phys. Rev. Lett.*, 77(18):3865–3868, October 1996.

[16] J. P. Perdew and Y. Wang. Accurate and simple analytic representation of the electron-gas correlation energy. *Phys. Rev. B*, 45(23):13244–13249, June 1992.

[17] W. Setyawan and S. Curtarolo. High-throughput electronic band structure calculations: Challenges and tools. *Comp. Mat. Sci.*, 49:299–312, 2010.

[18] H. Sowa. The high-pressure behavior of CdSe up to 3 GPa and the orientation relations between its wurtzite- and NaCl-type modifications. *Solid State Sci.*, 7:1384–1389, 2005.

[19] P. Villars and L.D. Calvert. *Pearson's Handbook of Crystallographic Data for Intermetallic Phases.* American Society for Metals, Materials Park, Ohio, 1st edition, 1985.

[20] P. Villars and J. L. C. Daams. Atomic-environment classification of the chemical elements. *J. Alloys Compd.*, 197:177–196, 1993.

[21] R. W. G. Wyckoff. *Crystal Structures*, volume 1. John Wiley & Son, Inc., Easton, PA, 2nd edition, 1963.
